# Supplementary material for: Entanglement between a photonic time-bin qubit and a collective atomic spin excitation
Source: arXiv:1801.05723 ancillary file (2018-01-17)
Supplement: Supplementary file 1 [file Supplemental_Material.pdf]

# Supplemental Material for:
# Entanglement between a photonic time-bin qubit and a collective atomic spin excitation

Pau Farrera,[1,*] Georg Heinze,[1,†] and Hugues de Riedmatten[1,2,‡]

[1] *ICFO-Institut de Ciencies Fotoniques, The Barcelona Institute of Science and Technology, 08860 Castelldefels (Barcelona), Spain*

[2] *ICREA-Institució Catalana de Recerca i Estudis Avançats, 08015 Barcelona, Spain*

In this document we give more details about theoretical concepts and technical issues of our experiment. In particular, we describe the spin-wave rephasing process, the effect of photons emitted in different transitions, and the calibration of the Mach-Zehnder interferometers.

PACS numbers: 03.67.-a, 03.67.Bg, 03.65.Ud, 42.50.-p

## PERIODIC REPHASING OF THE COLLECTIVE ATOMIC EXCITATION

As mentioned in the main text, one of the key features of our experiment is an homogeneous magnetic field that induces a periodic dephasing and rephasing of the collective atomic excitations. The detailed explanation of this process is the following. After optically pumping the atoms in state $|g\rangle = |5^2S_{1/2}, F = 1\rangle$, a write pulse with linear polarization parallel to the Y axis couples off-resonantly the $|g\rangle \rightarrow |e\rangle = |5^2P_{3/2}, F = 2\rangle$ transition. This polarization corresponds to a combination of $\sigma+$ and $\sigma-$ in our chosen frame of reference and couples the Zeeman sublevels shown in Fig. 1(b). Using a polarization beam splitter we couple into a single mode fiber write photons that are linearly polarized along the Z axis, which are generated from $\pi$ atomic transitions. The detection of a write photon heralds the presence of a collective atomic excitation (one atom in $|s\rangle = |5^2S_{1/2}, F = 2\rangle$) described by the following equation

$$|\Psi_a(t=0)\rangle = \frac{1}{\sqrt{N}} \sum_{j=1}^{N} e^{i(\mathbf{k}_W - \mathbf{k}_w)\mathbf{x}_j} |g_1 ... s_j ... g_N\rangle \quad (1)$$

where $N$ is the total number of atoms, $\mathbf{x}_j$ the position of atom in $|s\rangle$, and $\mathbf{k}_{\mathrm{W(w)}}$ the wavevector of the write pulse (photon).

The time evolution of the previous state under the presence of a magnetic field B can be obtained from the Schrödinger equation

$$|\Psi_{\mathrm{a}}(t)\rangle = \frac{1}{\sqrt{N}} \sum_{j=1}^{N} e^{i(\mathbf{k}_{\mathrm{W}} - \mathbf{k}_{\mathrm{w}})\mathbf{x}_j + i\int_0^t \Delta w_j(t')dt'} |g_1 ... s_j ... g_N\rangle \quad (2)$$

$$= \frac{1}{\sqrt{N}} \sum_{j=1}^{N} e^{i(\mathbf{k}_{\mathrm{W}} - \mathbf{k}_{\mathrm{w}})\mathbf{x}_j + i\Delta w_j t} |g_1 ... s_j ... g_N\rangle \quad (3)$$

where $\Delta w_j$ is the relative detuning of each of the states $|g_1 ... s_j ... g_N\rangle$ [1]. These detunings depend on the Zeeman sublevels $m_{F=1}$ and $m_{F=2}$ involved in each excitation path shown in Fig. 1(b). They are given by $\Delta w_j = \mu_{\mathrm{B}} B(g_{F=2}m_{F=2} - g_{F=1}m_{F=1})/\hbar$ where $\mu_{\mathrm{B}}$ is the Bohr magneton, $B$ is the magnetic field, $g_{F=1(2)}$ is the Landé g-factor and the $m_{F=1(2)}$ quantum number corresponding to the z-component of the total angular momentum. Please note that in Eq. 3 we did not consider the sate evolution due to other effects (e.g. atomic motion), as we expect them to change the state on a much longer time scale that the one used in this experiment (c.f. green open circles in Fig.2(a) of the main text).

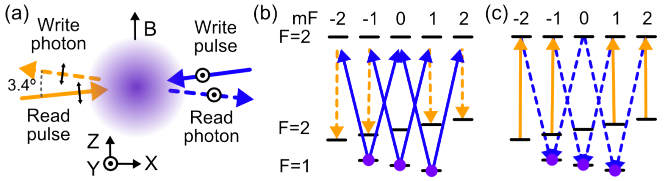


FIG. 1. (color online) (a) Schematic drawing of the atomic cloud and the four light fields involved in the entanglement generation process. The black arrows and dots above the optical beams represent their polarization. (b-c) Atomic levels with the coupled optical transitions for the write process (b) and the read process (c). The Zeeman splitting of the excited state is not shown in order to avoid any confusion with the transition detunings.

The probability to convert the collective excitation into a single read photon $p_{(\mathrm{r|w})}$ should be proportional to the overlap between the original spin-wave state and the state at the readout time $p_{(\mathrm{r|w})}(t_{\mathrm{R}}) \propto |\langle\Psi_{\mathrm{a}}(t=0)|\Psi_{\mathrm{a}}(t=t_{\mathrm{R}})\rangle|^2$. This leads to the following expression

$$p_{(\mathrm{r|w})}(t) \propto \left| \sum_{k=0}^{3} P_k e^{-i\Delta w_k t} \right|^2 \quad (4)$$

where the different values of k represent the four different excitation paths, and the coefficients $P_k$ correspond to the ratio of atoms that contributed to each path.

To fit the data in Fig. 2(a) of the main text we use

Eq. 4 multiplied by a proportional factor $C_\mathrm{p}$ and with an added offset $C_\mathrm{o}$. The proportional factor $C_\mathrm{p}$ accounts for the effects different to spin-wave dephasing that decrease the value of $p_{(\mathrm{r}|\mathrm{w})}$ in our experiment. This includes the imperfect fiber coupling efficiency or the detection in the write process of photons emitted in the $|e\rangle \rightarrow |g\rangle$ transition leading to wrong heralding events. The offset factor $C_\mathrm{o}$ includes detector dark counts and the amount of undirectionally emitted photons that are coupled to the read photon fiber and detected. The expression of coefficients $\Delta w_k$ is mentioned before and from the values given by the fit we obtain the homogeneous magnetic field value $B = 2.1\,\mathrm{G}$ mentioned in the main text.

## DISCUSSION OF THE IMPERFECTIONS IN THE READ-OUT PROCESS

As mentioned in the main text, one detrimental effect in our read-out process is that the early read pulse scatters late atomic excitations. This is the reason that the early read pulse has an area of $\pi/2$, while the area of the late read pulse is $\pi$. This imperfection in the read-out process is equivalent to an optical loss, which can be modelled by a beam splitter where one of the two outputs is lost. If the loss is the same for both time-bins, only the efficiency of the process is affected, but not the fidelity post-selected upon a photon coincidence detection (assuming low $P_\mathrm{W}$). To explain this in more detail we now describe the four different processes that could happen in an ideal scenario of the read-out process:

1 - A spin excitation was generated in the early bin and the early read pulse converts in into a photon.

2 - A spin excitation was generated in the early bin and the early read pulse does not convert it into a photon (in this situation the late read pulse will convert the excitation into a photon with undirectional emission).

3 - A spin excitation was generated in the late bin and the early read pulse converts it into a photon (in this situation the early read pulse will convert the excitation into a photon with undirectional emission).

4 - A spin excitation was generated in the late bin and the early read pulse does not convert it into a photon.

Processes 1 and 4 lead to a directional emission of a read photon, and form a quantum superposition in the form of an entangled state between the write and read photons. They correspond to a successful transfer of the atomic quantum state to the read photon. We make interfere in the interferometer the photons generated by processes 1 and 4 in order to characterize the entangled state.

Processes 2 and 3 will lead the generation of photons with undirectional emission, since in these situations the spin excitations are completely dephased (this can be seen in Fig. 1c from the main text). The fraction of these photons that are coupled in the read photon fiber and detected affect the selectivity and therefore the entanglement fidelity (or the Bell parameter). However the impact of the undirectional photons decreases when the write power is decreased (as observed in fig 2b from the main text). Therefore for sufficiently low write pulse power, their impact can be considered negligible.

## DETECTION NOISE FILTERING AND CHARACTERIZATION

In order to separate the write (read) photons from the write (read) pulses light we used two different methods:

1 - Spatial filtering: the spatial modes of the pulses and the photons have an angular separation of 3.4° as it is shown in Fig. 1(a).

2 - Since the photons exhibit orthogonal polarizations with respect to the pulses (see also Fig. 1(a)), we can apply polarization filtering using polarizing beam splitters (PBSs). We placed PBSs in front of the write and the read photon couplers.

In this situation, the probabilities to detect a noise photon in any of the write photon detectors ($\mathrm{D}_\mathrm{w}^+$ and $\mathrm{D}_\mathrm{w}^-$) is $p_\mathrm{Nw} = 6 \cdot 10^{-6}$ and $p_\mathrm{Nr} = 8 \cdot 10^{-5}$ in the read photon detectors. The probability to detect a coincidence due to noise ($p_\mathrm{Nw} \cdot p_\mathrm{Nr}$) is then much lower than the typical write-read photon coincidence detection probabilities (i.e. $p_\mathrm{wr} \approx 10^{-6}$ for $P_\mathrm{W} \approx 8\ \mu\mathrm{W}$).

## SINGE PHOTON INTERFERENCE OF THE WRITE AND READ PHOTONS

As shown in Fig. 2(b) of the main text, we observe strong photon correlations between both early and both late write and read photonic bins. This means that by measuring one of the photonic modes (either the write or the read) one could get information about the temporal bin of the other mode. A consequence is that we should not see single photon interference when the two bins of one mode are overlapped in the interferometer. However, as shown in Fig. 2 we do observe single photon interference. In this figure we show the number of read photons detected in detectors $D_\mathrm{r}^+$ (blue dots) and $D_\mathrm{r}^-$ (green circles) for the measurement shown in Fig. 3(c) of the main text. They correspond to all counts in the read photon central bin shown in Fig. 3(a) of the main text. They oscillate with a visibility of $V \approx 24\%$ when the read photon interferometer phase is changed by the voltage $U_\mathrm{r}$ applied to its piezo fiber stretcher. When scanning the voltage of the write piezo stretcher, we also observe single photon interference in the write mode with a similar visibility ($V \approx 23\%$).

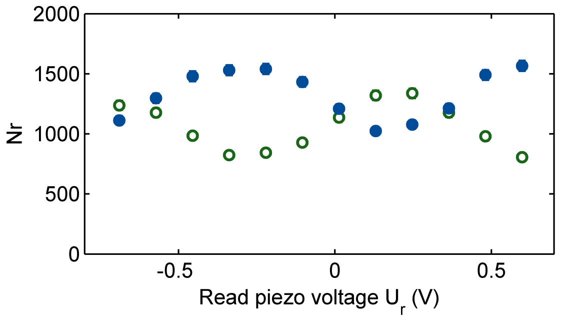


FIG. 2. (color online) Number of detected read photons (Nr) as a function of the piezo voltage of the read interferometer. The blue dots and the green open circles represent the counts detected at each of the two outputs of the read interferometer in detectors $D_r^+$ and $D_r^-$ (see Fig.1 in the main text).

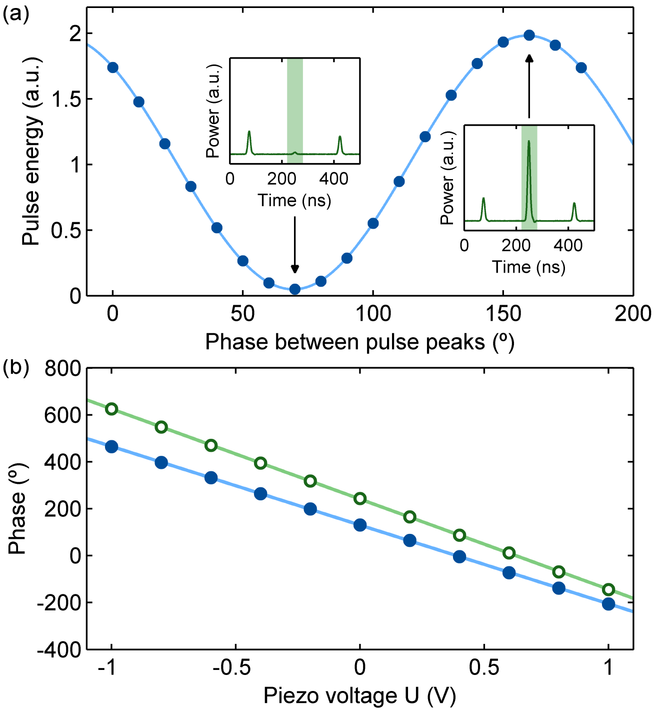


FIG. 3. (color online)(a) Write interferometer characterization with bright pulses mimicking the write photons analysed in the experiment. The insets show the temporal profile of the light fields at the output of the interferometer. The blue points show the output energy of the central bin. (b) Phase of the interference fringe shown in (a) as a function of the voltage applied to the piezo fiber stretcher. The blue dots correspond to data of the write interferometer and the green open circles correspond to the read interferometer.

We attribute this effect to write photons that are emitted in the $|e\rangle \rightarrow |g\rangle$ transition and read photons emitted in the $|e\rangle \rightarrow |s\rangle$ transition. These photons are not part of the entangled state that is described in the main text and represent noise that decreases the entanglement fidelity. Nevertheless since these photons do not show write-read photon correlations, their impact in the correlation parameters E (which are calculated from write-read photon coincidence probabilities) is very low. Due to the fact that the frequency of these photons is 6.8 GHz away from the one of the entangled write and read photons, they could be filtered by Fabry-Perot cavities as used in previous works [1]. However, in this experiment we did not use spectral filtering in order to have higher photon detection rates and hence reduce the effect of long term instabilities.

## CHARACTERIZATION OF THE MACH-ZEHNDER INTERFEROMETERS

As explained in the main text, the phase delay between the two paths of the interferometers can be controlled by a piezo-electric ceramic cylinder that has a section of fiber rolled around. Applying a voltage to this piezo-electric device induces a stretching to the rolled fiber changing its optical path length. We use this capability for two purposes: (1) to lock the interferometer phase during the atomic cloud preparation time, and (2) to set later the qubit basis phase during the entanglement generation time. In order to know which voltages we need to apply to obtain the desired phase delays, we characterized the interferometers with bright laser light pulses.

We used light pulses with similar characteristics as the doubly peaked write and read photons. The measured pulses at the output of the write interferometer are shown in the insets of Fig. 3(a) for two values of the phase difference between the two input pulse peaks. The total energy of the central output peak as a function of the phase difference between the two input pulse peaks is represented as blue points in Fig. 3(a). The oscillation shows a visibility of $V = 95\,\%$ which we expect to be limited by the linewidth of the two lasers used for the pulses and the interferometer lock light.

The phase of the resulting interference fringes is shown in Fig. 3(b) for different voltages applied to the corresponding piezo-electric fiber stretchers. The blue dots represent the data obtained from the write photon interferometer, while the green open circles are obtained from the read photon interferometer.

The linear fits of the calibration data give a relation of $-335.4\,°/\mathrm{V}$ and $-384.4\,°/\mathrm{V}$ for the write and read interferometers, respectively. These values are used to obtain the voltages which are set in the CHSH Bell inequality measurement.

* Contact: pau.farrera@icfo.eu
† Contact: georg.heinze@icfo.eu
‡ http://qpsa.icfo.es

[1] B. Albrecht, P. Farrera, G. Heinze, M. Cristiani, and H. de Riedmatten, Phys. Rev. Lett. **115**, 160501 (2015).
